# Supplementary material for: Effective Seed Scheduling for Fuzzing with Graph Centrality Analysis
Source: arXiv:2203.12064 source file (2022-03-24)
Supplement: Supplementary file 1 [file appendix_bk.tex]

\appendix
\subsection{Major Revision List of Changes}
We summarize how we have addressed the requested changes in our major revision below. We also colored the corresponding text \revise{blue} in the paper for clarity. 

\medskip
\noindent
\textbf{Additional statistical techniques in our evaluation.}

In Section \ref{evaluation}, our results (e.g., Tables \ref{tab:libfuzzer_cov}, \ref{tab:afl_cov}) now include performance comparisons in terms of arithmetic mean and median and are normalized appropriately. In addition, we ran the edge coverage experiments a total of 10 times and use the Mann Whitney U test to determine statistical significance of our results (Tables~\ref{tab:libfuzzer_covp_1h}, ~\ref{tab:libfuzzer_covp},~\ref{tab:afl_p_1h},~\ref{tab:afl_p_24h}). We planned to perform k-fold cross validation to select $\alpha$, but we later realized that performing k-fold cross validation over only 12 data points (e.g., 12 FuzzBench programs) will not be statistically meaningful. Therefore, instead of the k-fold cross validation experiment, we measure the effect of different $\alpha$ parameter settings on \ToolName{} reported in Table~\ref{tab:aba_alpha} and selected $\alpha$ based on these results.

\medskip
\noindent
\textbf{Updated edge coverage experiments.}
We have improved our edge coverage experiments in Section \ref{evaluation} by evaluating all tested seed schedulers over the same 12 diverse, real-world programs from Google FuzzBench listed in Table~\ref{tab:libfuzzer_cov}. We also compared against input prioritization techniques by using TortoiseFuzz as seen in Table~\ref{tab:afl_cov_1h} and Table~\ref{tab:afl_cov}. Lastly, given \ToolName{} uses two separate processes, in our experiments, we assigned AFL/Libfuzzer the exact same amount of computation that \ToolName{} utilizes to keep the comparison fair. 

Moreover, we greatly reduced our prototype's overhead since the time of our original submission. Instead of caching the edge horizon graph, our initial prototype naively built the entire edge horizon graph from scratch for each centrality computation, which contributed significantly to its overheads. Our improved prototype now caches the edge horizon graph. This performance optimization significantly reduced our overheads from $<15\%$ to $<1\%$ in arithmetic mean reported in Table \ref{tab:libfuzzer_runtime}. Note this cached graph is not static: \ToolName{} periodically updates it by deleting visiting nodes as described in Section~\ref{methodology}.

%Lastly, we note that we planned to use only the 12 FuzzBench programs in our entire evaluation, but this choice would have required us to drop our original submission's bug finding experiments, which used another set of 12 real-world programs listed in Table~\ref{tab:studied_programs}. Therefore, we keep all 24 programs but use the 12 FuzzBench programs for all our evaluation except the bug-finding experiments. 

\medskip
\noindent
\textbf{Bug reporting.}
In Section \ref{evaluation} RQ2, we added step-by-step details of our bug triaging process, where we de-duplicate crashes based on AFL-Cmin and unique stack traces followed by manual investigation of the source code. We did not report the unique bug count as there was concern among the reviewers that it may be misleading (see revision comments). 

\medskip
\noindent
\textbf{Related work.}
We added 6 more input prioritization and seed scheduling references to our related work in Section~\ref{related_work}. We also compare and contrast \ToolName{} with \texttt{SAVIOR}.

\medskip
\noindent
\textbf{Additional experiments.}
Besides our improved edge coverage experiments, we have added 4 new experiments to our design choice experiments in Section \ref{evaluation}, which we now conduct over all 12 Google FuzzBench programs. The order corresponds to the order of revision requirements for clarity.
\begin{enumerate}

    \item Table~\ref{tab:aba_alpha} shows the effect of $\alpha$ on \ToolName{}. 
    \item In Table~\ref{tab:aba_ranking}, we compare the correlation between \ToolName{}'s per-node ranking to the ranking of the ideal strategy that counts the number of feasible and reachable edges from a node.
    \item Table~\ref{tab:aba_cent} shows the effect of different centralities on \ToolName{}. 

    \item Table~\ref{tab:aba_loop} shows the effect of loop removal on \ToolName{}.
\end{enumerate}

\medskip
\noindent
\textbf{Writing Changes.}
The order corresponds to the order of revision requirements for clarity. 
\begin{enumerate}
    %\item In Section \ref{background}, we provide intuition how $\alpha$ may be useful. 
     \item In Section \ref{evaluation}, we updated the result box to distinguish between graph analysis overheads and fuzzer overheads in the Runtime Overhead RQ. We also added a comment about the increased performance overhead of fuzzing generally being acceptable in practice. 
    \item In Section \ref{evaluation}, we dropped our original comments about configuring the fuzzers to use havoc mode because we now use Google FuzzBench with its default settings and configuration, which uses havoc mode by default~\cite{FuzzBench}.  
    %using havoc mode  \cite{FuzzBench} \dongdong{add a line to say havoc mode is the default setting in FuzzBench dataset}
    \item In Section \ref{evaluation}, we used the term impact of design choices.
    \item In Section \ref{evaluation}, we clarified our experimental setup of concolic execution seed scheduling.
    
    \item In Section \ref{methodology}, we simplified the discussion about edge horizon graph transforms. We now only use a single graph transform that removes loops compared to our original submission which used multiple transforms.
    \item In Section \ref{implementation}, we discussed limitations of our prototype such as not handling indirect calls. We also discuss potential implications of such imprecision on \ToolName{}.
    \item In Section \ref{methodology}, we clarified centrality is re-computed, that is, after a fixed time elapses or the fuzzer discovers new edge coverage. 
   
\end{enumerate}

%\abhi{should we move bug finding to Appendix? and drop description from abstract/Introduction? @Suman}
